# Supplementary material for: Online Video Understanding: OVBench and VideoChat-Online
Source: arXiv:2501.00584 source file (2025-04-17)
Supplement: Supplementary file 1 [file supp_benchmark.pdf]

# [SP] Spatial Perception

**Question:** Based on visible information, which option most accurately describes **the location of the hats** on the screen? (Note: Positions with counts, e.g., 'left-middle (2)', indicate multiple objects in the same area.)?

**Timestamp:** 31.0s

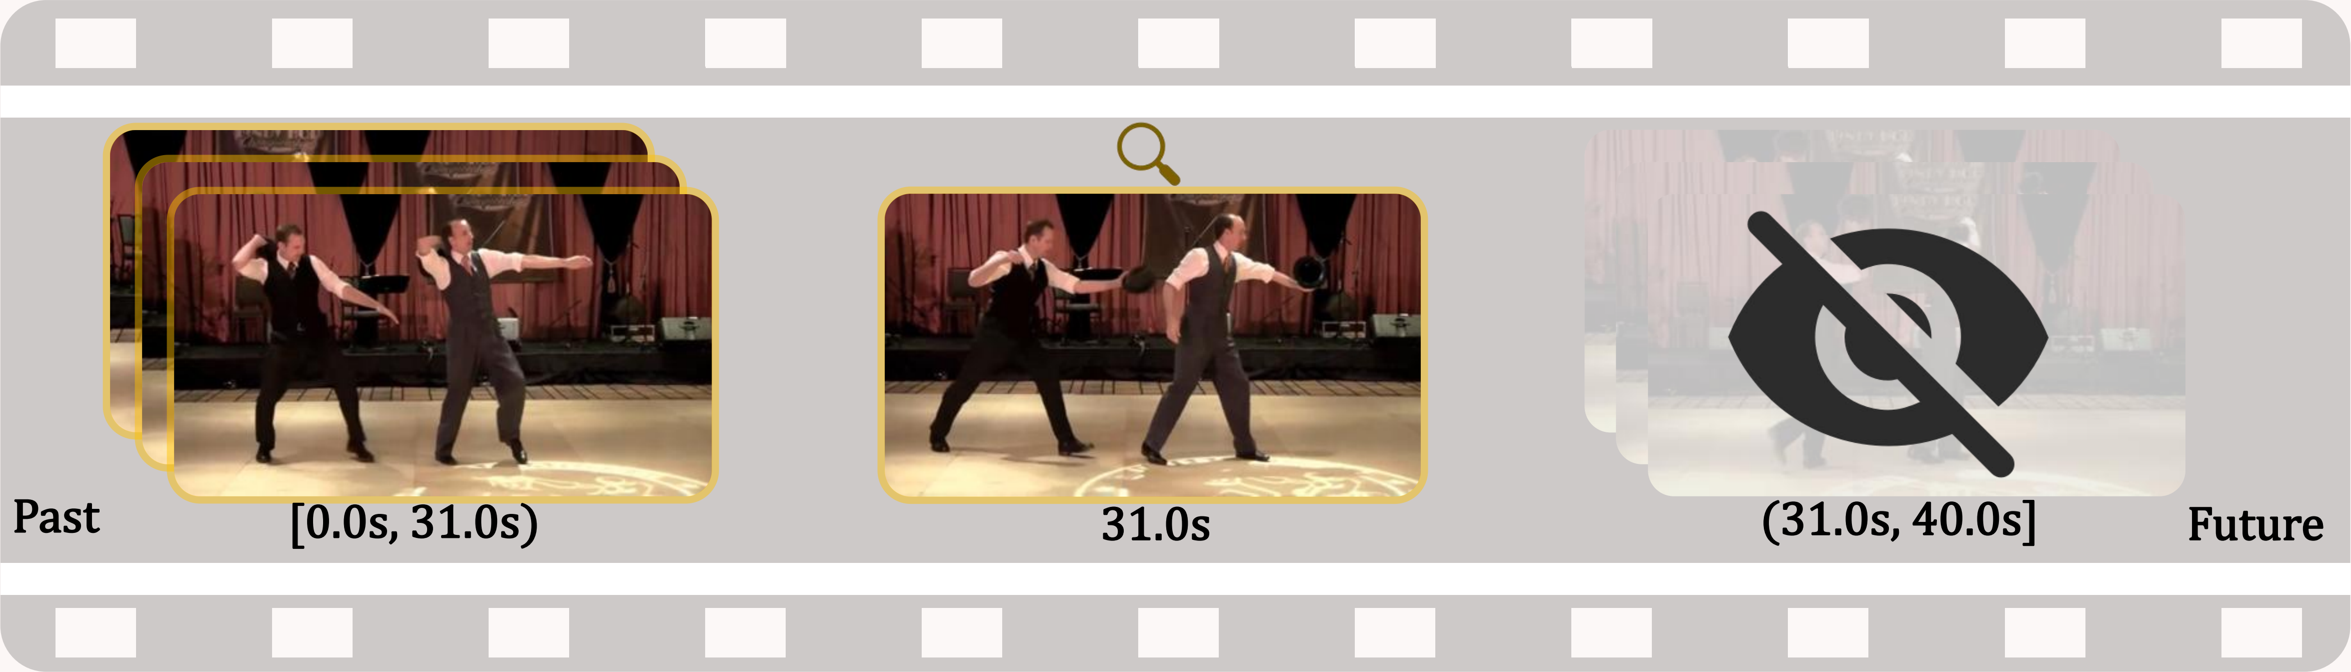


**Options:**

(A) right-middle, right-middle, left-bottom, left-middle (2)

(B) center, left-top, left-bottom (2)

(C) left-middle, left-middle (2), left-top

(D) right-top, top

**Correct Answer**: (D)

# [STP] Spatial Temporal Perception

**Question:** Compared with 34 seconds ago, are the calf [0.177, 0.289, 0.409, 0.6] and the calf [0.635, 0.629, 1.0, 1.0] closer or farther apart?

**Timestamp:** 38.0s

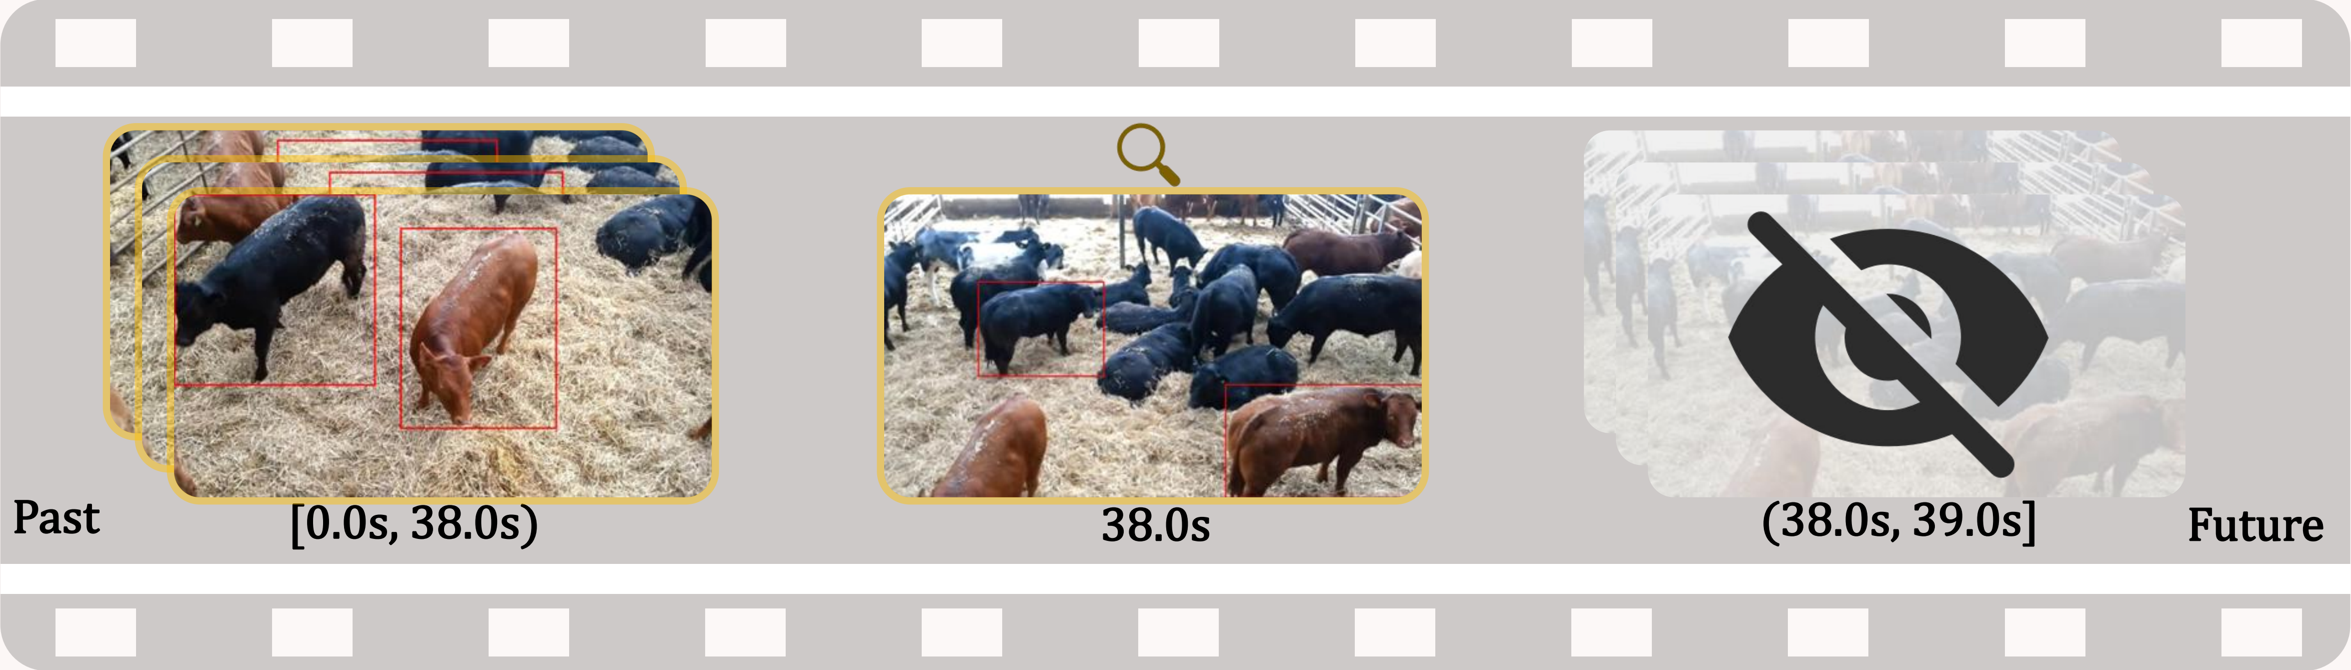


**Options:**

(A) Their distance almost remains unchanged

(B) They are getting farther apart.

(C) They are getting closer

**Correct Answer**: (B)

# [TP] Temporal Perception

**Question:** How long has the person in the scene been performing the 'put up to the corner'?
**Timestamp:** 66.0s

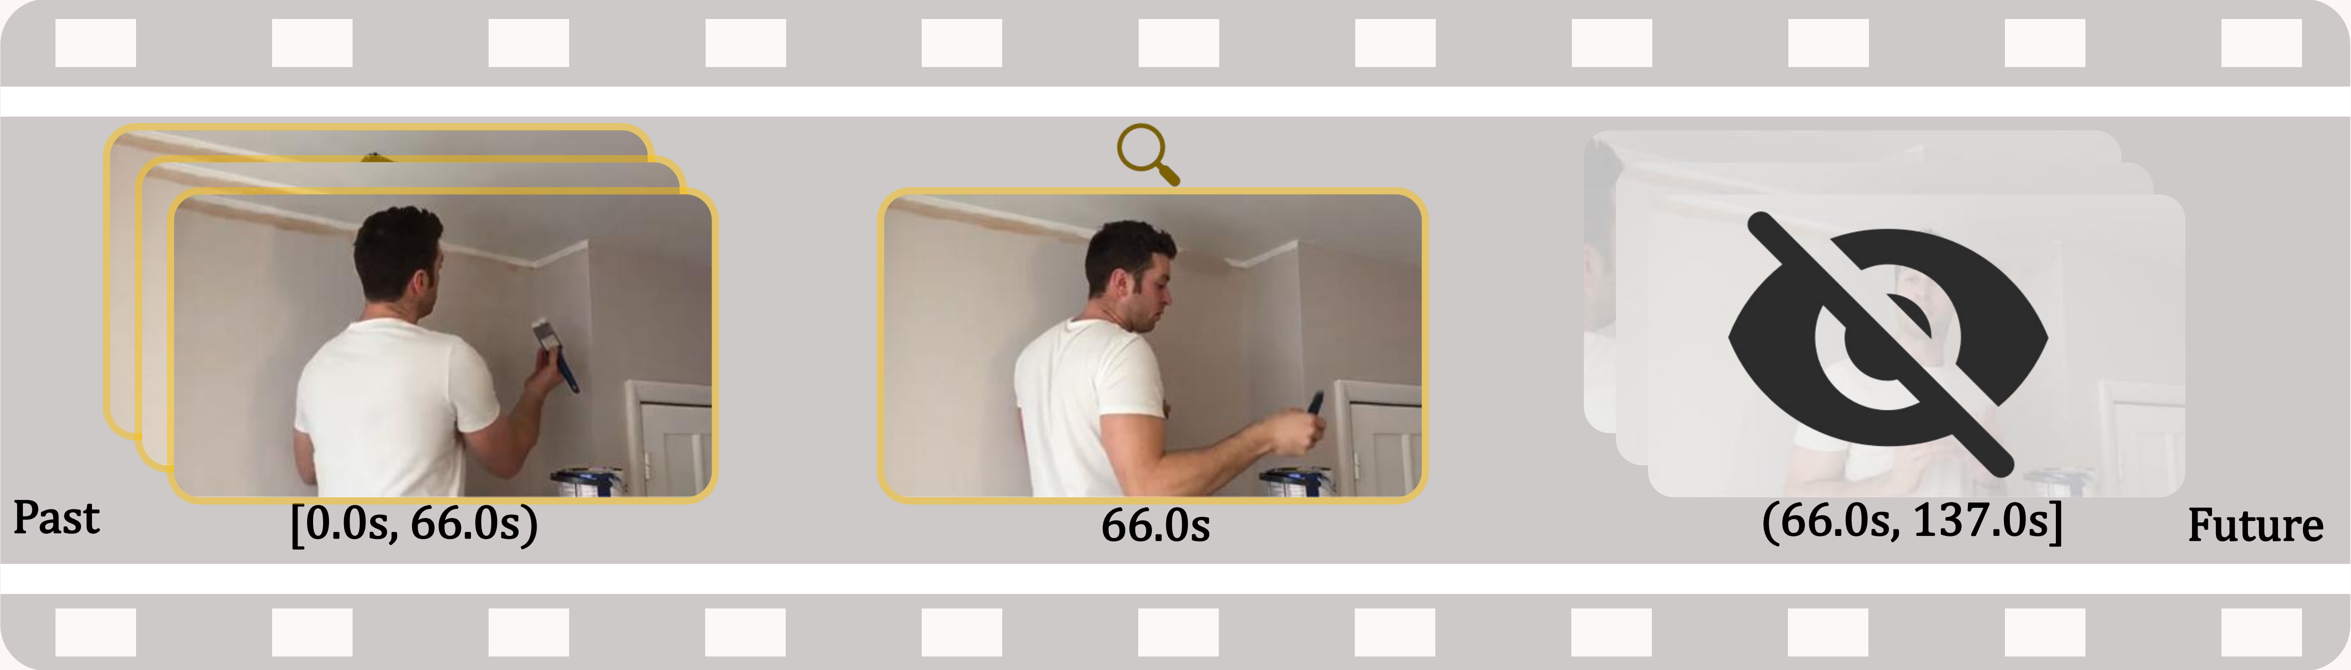


**Options:**
(A) 27~28s (B) 31~32s
(C) 5~6s (D) 10~11s

**Correct Answer**: (D)

# Hallucination

**Question:** Is the person in the current frame still performing the 'put stick on lemon’?
**Timestamp:** 65.0s

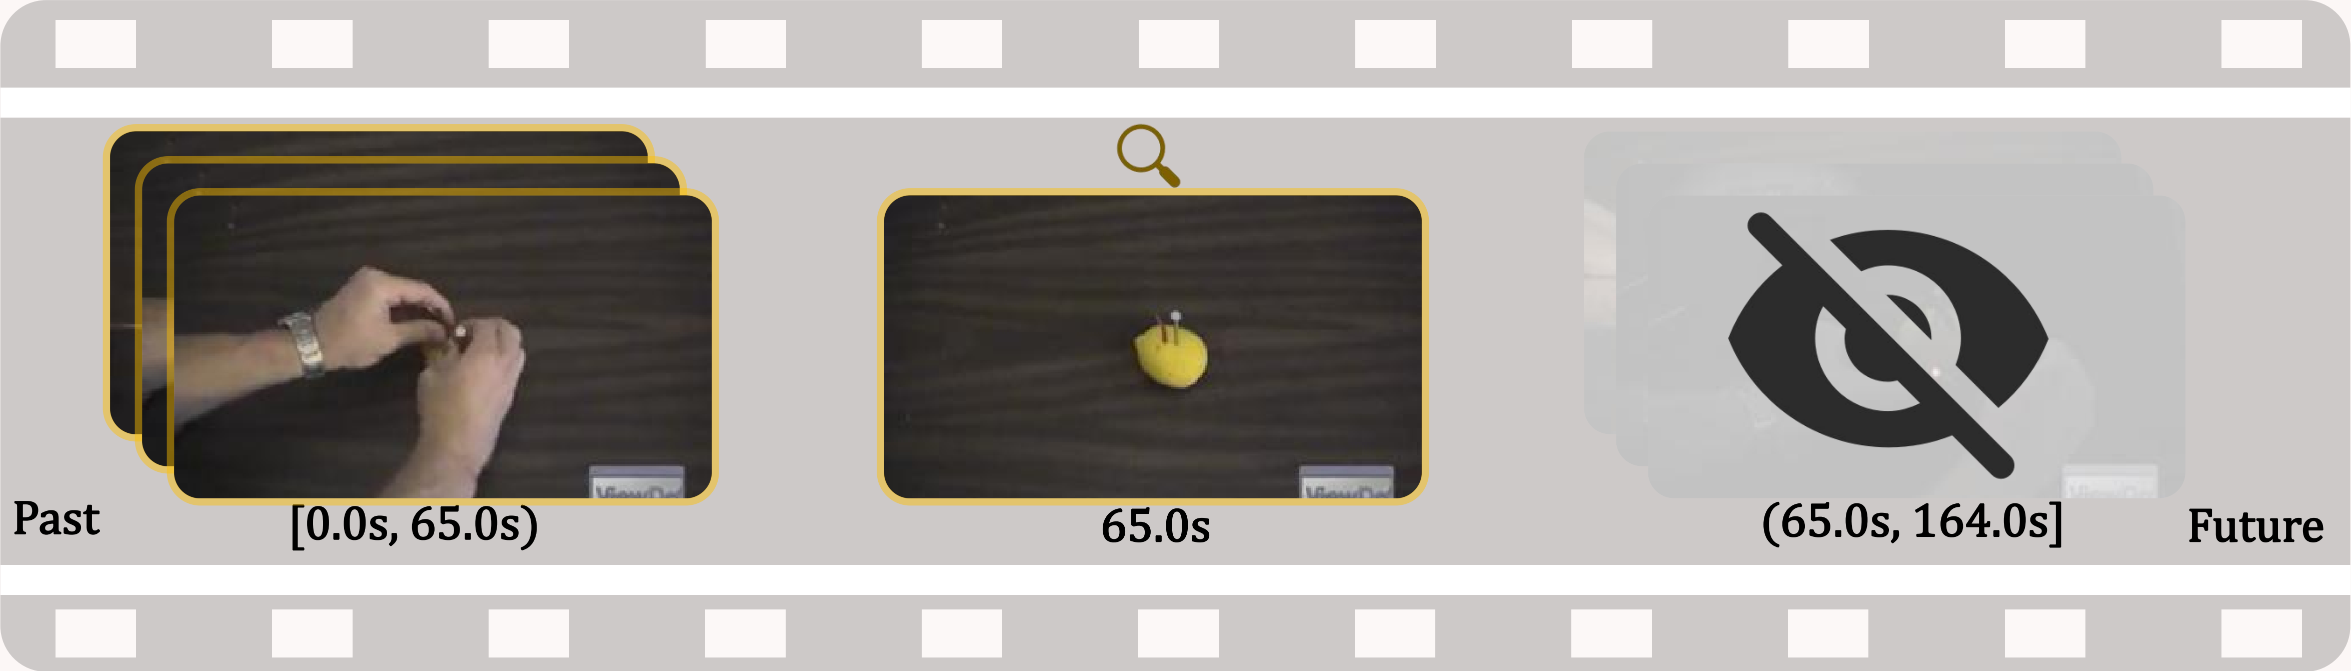


**Options:**

(A) Yes (B) No

**Correct Answer**: (B)

# [PM] Past Memory

**Question:** What actions did the person not perform in the last 150 seconds?
**Timestamp:** 205.0s

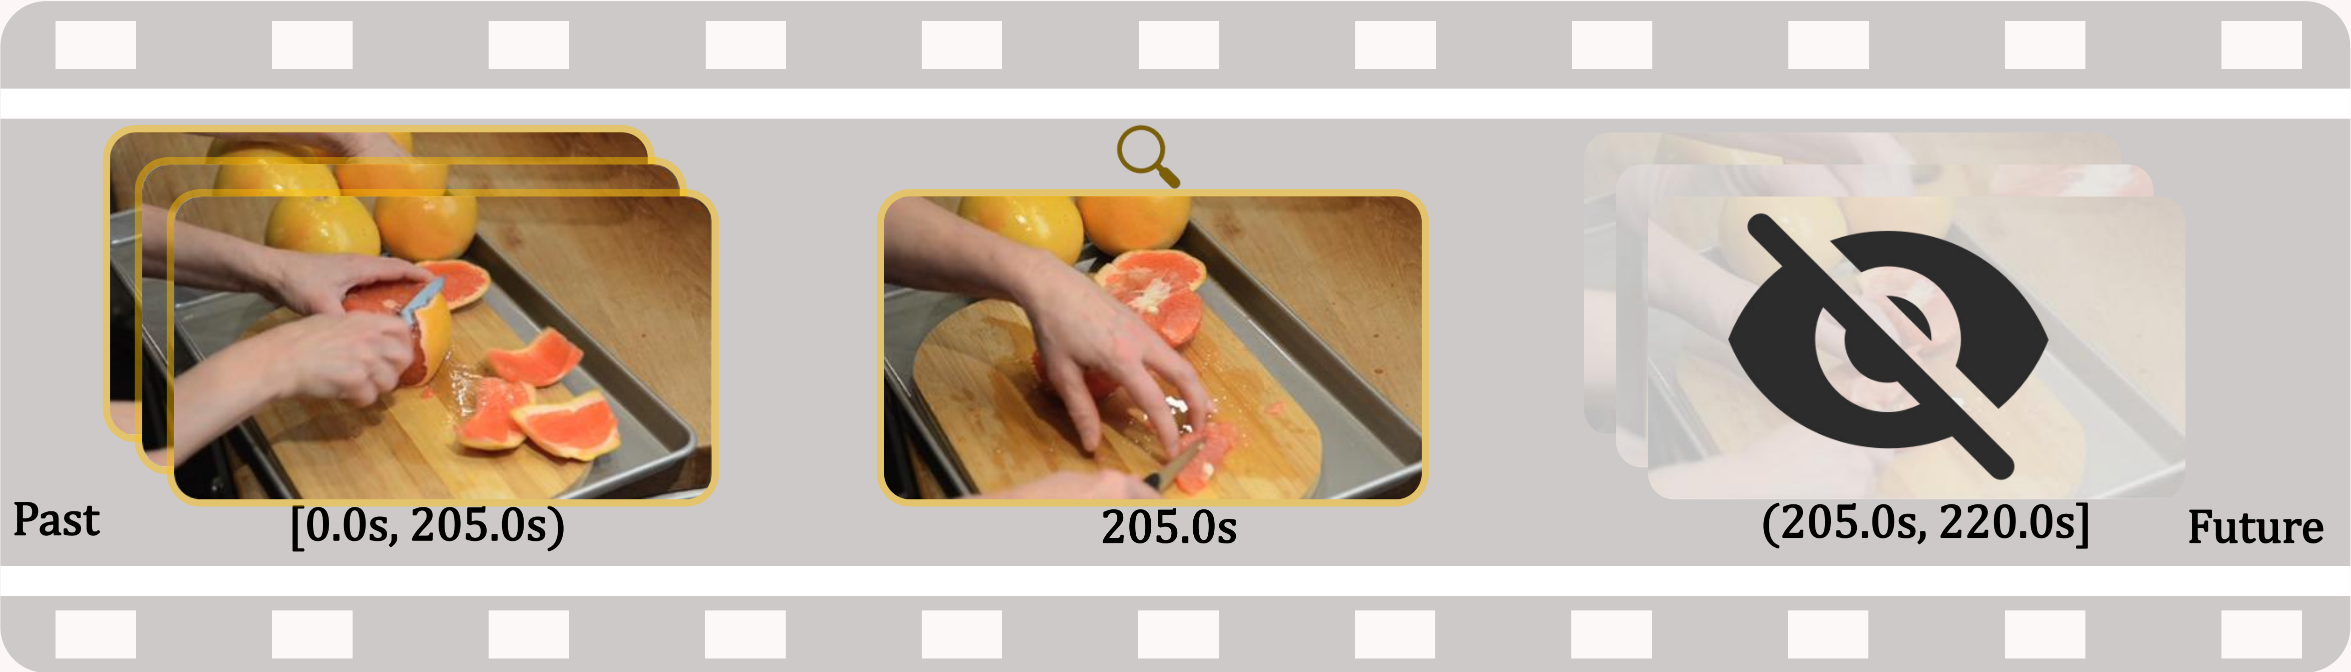


**Options:**

(A) remove the peel
(B) cut in half
(C) cut both ends and remove fruit seeds
(D) slice the pulp

**Correct Answer**: (B)

# [FP] Future Prediction

**Question:** My goal is 'paste Window Decal'. What are the next steps I should take?
**Timestamp:** 91.0s

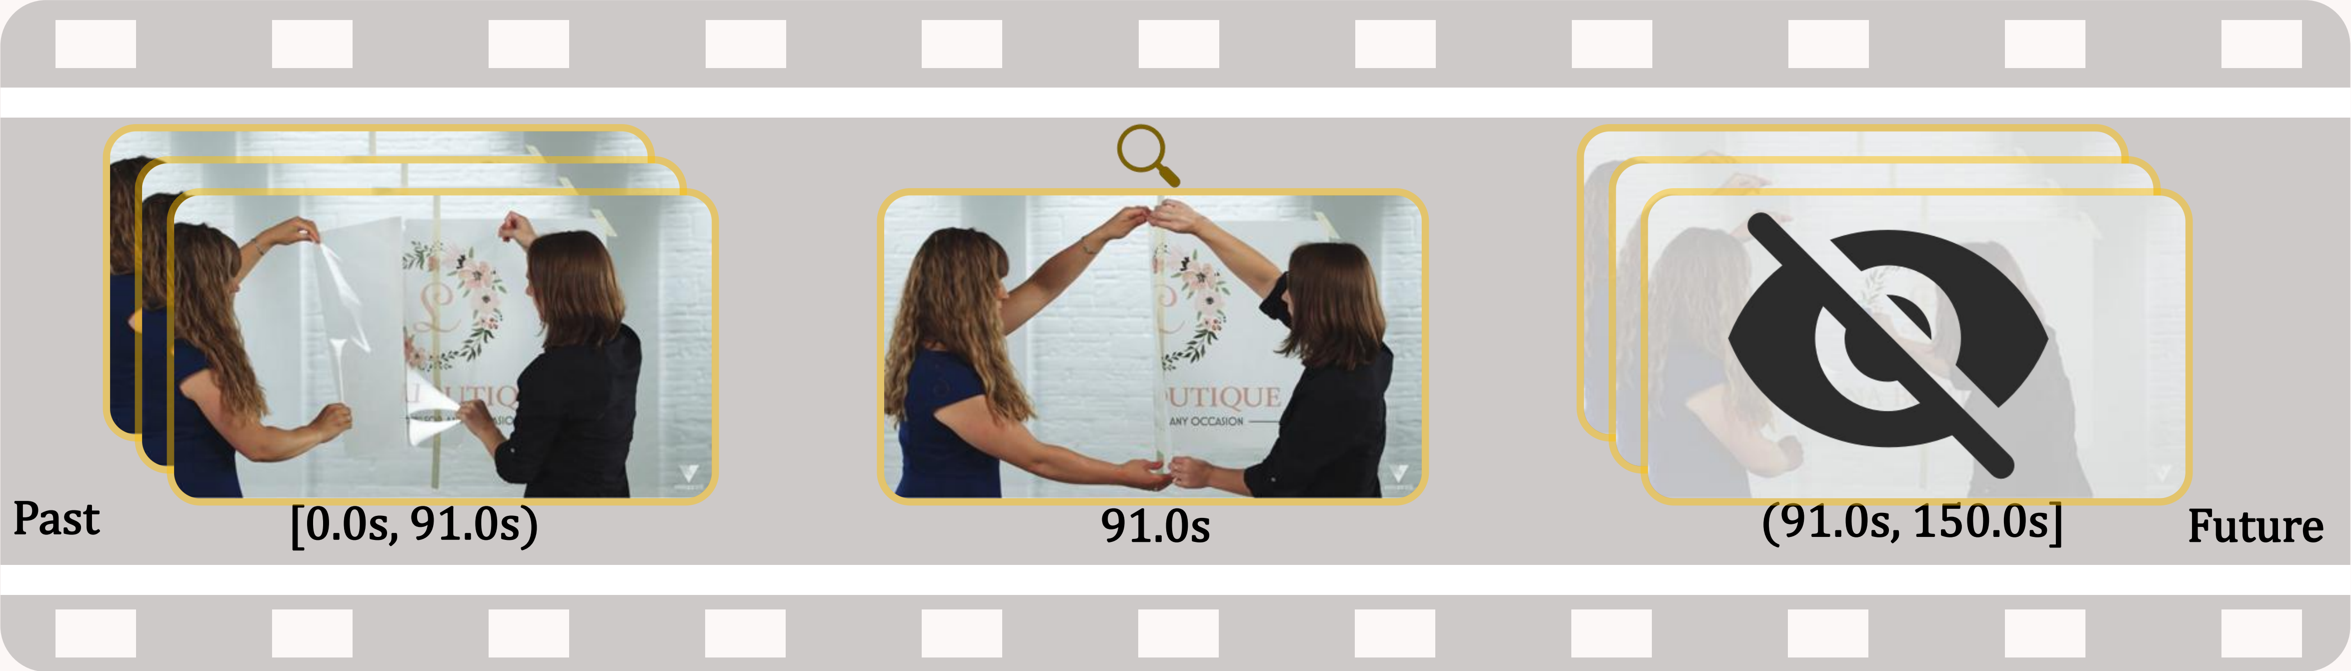


**Options:**

(A) apply soap water to the glass surface
(B) press the decal
(C) tear off the other side of the decal
(D) align the position

**Correct Answer:** (B)
