# Supplementary material for: Online Video Understanding: OVBench and VideoChat-Online
Source: arXiv:2501.00584 source file (2025-04-17)
Supplement: Supplementary file 2 [file supp_benchmark_results.tex]

%usepackage{adjustbox}
\begin{table*}[]
    \centering
    \resizebox{\textwidth}{!}{%
    \begin{tabular}{lllllllllllllllllll}
    \toprule 
    Task   Name                 & \multicolumn{1}{c}{}                                     & \multicolumn{3}{c}{FP}                                                  & \multicolumn{3}{c}{THV}                                                    & \multicolumn{3}{c}{PM}                                                  & \multicolumn{2}{c}{SP}                        & \multicolumn{2}{c}{STP}                         & \multicolumn{3}{c}{TP}                                                  & \multicolumn{1}{c}{}                      \\
    \cmidrule(lr){3-5} \cmidrule(lr){6-8} \cmidrule(lr){9-11} \cmidrule(lr){12-13} \cmidrule(lr){14-15} \cmidrule(lr){16-18}
    Subset Name                 & \multicolumn{1}{l}{\multirow{-2}{*}{Size}}           & \FPava & \FPevent & \FPtao & \Halava & \Halevent & \Haltao & \PMava & \PMevent & \PMtao & \SPava & \SPtao & \STPava & \STPtao & \TPava & \TPevent & \TPtao & \multicolumn{1}{c}{\multirow{-2}{*}{AVG}} \\
    \midrule
    \multicolumn{3}{l}{\cellcolor{gray!30}{\textit{sliding window size=32s fps=2}}}           & \cellcolor{gray!30}{}               & \cellcolor{gray!30}{}             & \cellcolor{gray!30}{}              & \cellcolor{gray!30}{}                & \cellcolor{gray!30}{}              & \cellcolor{gray!30}{}             & \cellcolor{gray!30}{}               & \cellcolor{gray!30}{}             & \cellcolor{gray!30}{}             & \cellcolor{gray!30}{}             & \cellcolor{gray!30}{}              & \cellcolor{gray!30}{}              & \cellcolor{gray!30}{}             & \cellcolor{gray!30}{}               & \cellcolor{gray!30}{}             &     \cellcolor{gray!30}{}                                      \\
    \midrule
    Gemini-1.5-Flash~\cite{gemini}           & \multicolumn{1}{c}{-}                                    & 71.4                  & 53.6                    & 21.9                  & 56.5                   & 60.8                     & 40.6                   & 36.7                  & 47.9                    & 62.5                  & 32.3                  & 37.5                  & 87.0                   & 50.0                   & 83.3                  & 22.3                    & 46.9                  & 50.7                                      \\
    % \midrule
    %            &                                     &                  &                    &                  &                   &                     &                   &                  &                    &                  &                  &                  &                   &                   &                  &                    &                  &                                      \\ 
    \midrule
    InternVL2~\cite{chen2023internvl}                   & 7B                                                       & 52.6                  & 60.2                    & 27.6                  & 57.5                   & \cellcolor{gray!30}{52.0}                     & 58.5                   & \cellcolor{gray!30}{38.8}                  & \textbf{67.1}                    & 58.3                  & 38.1                  & \textbf{31.3}                  & 87.4                   & 37.0                   & \cellcolor{gray!30}{75.4}                  & \cellcolor{gray!30}{31.4}                    & 5.9                   & 48.7                                      \\
    InternVL2~\cite{chen2023internvl}                   & 4B                                                       & 57.7                  & 57.0                    & 14.4                  & 59.2                  & 49.4                     & \cellcolor{gray!30}{60.0}                   & 30.3                  & 61.8                    & 46.3                  & 30.9                  & 20.1                  & 83.0                   & 32.3                   & 70.7                  & 29.4                    & 3.4                   & 44.1                                      \\
    LLaMA-VID~\cite{llamavid}                   & 7B                                                       & 43.6                  & 50.9                    & 19.6                  & \cellcolor{gray!30}{64.0}                   & 47.5                     & 46.8                   & 29.4                  & 48.9                    & 51.2                  & 31.9                  & 11.2                  & 75.7                   & 24.8                   & 59.1                  & 26.0                    & \cellcolor{gray!30}{40.0}                  & 41.9                                      \\
    LLaVA-Onevision~\cite{LLaVA-OneVision}             & 7B                                                       & \textbf{68.0}                  & 62.7                    & \textbf{35.9}                  & 58.4                   & 50.3                     & 46.5                   & 29.4                  & 60.7                    & 58.0                  & \textbf{43.1}                  & 14.2                  & 86.5                   & \cellcolor{gray!30}{49.7}                   & 70.7                  & 28.1                    & 30.2                  & 49.5                                      \\
    LongVA~\cite{longva}                        & 7B                                                       & 64.1                  & 56.5                    & \cellcolor{gray!30}{29.5}                  & 54.9                   & 51.9                     & 34.8                   & 35.3                  & 55.6                    & 57.7                  & 31.6                  & 3.4                   & 67.4                   & 44.7                   & \textbf{80.0}                  & 26.7                    & 4.0                   & 43.6                                      \\
    MiniCPM-V2.6~\cite{hu2024minicpm}                & 7B                                                       & 33.3                  & 35.9                    & 15.0                  & 59.2                   & 50.8                     & 55.1                   & 25.0                  & 37.4                    & 41.7                  & 26.6                  & 11.8                  & \textbf{98.3}                   & 36.3                   & 66.1                  & 26.4                    & 6.2                   & 39.1                                      \\
    Qwen2-VL~\cite{wang2024qwen2vl}                   & 7B                                                       & \cellcolor{gray!30}{60.3}                  & \textbf{66.1}                   & 22.1                  & 54.9                   & 51.5                     & 51.1                   & 37.8                  & \cellcolor{gray!30}{64.4}                    & \cellcolor{gray!30}{69.3}                  & 35.3                  & 28.5                  & \cellcolor{gray!30}{97.0}                   & 49.4                   & 65.1                  & 30.8                    & 11.7                  & \cellcolor{gray!30}{49.7}                                      \\
    \textcolor{red}{LITA}~\cite{huang2025lita}                          & 7B                                                       &19.2	&24.5	&19.9	&40.8	&48.9	&24.9	&3.1	&27.3	&6.4	&6.9	&14.6	&35.2	&23.9	&27.4	&0.5	&3.4	&20.4

                     \\
    \textcolor{red}{TimeChat}~\cite{timechat}                    & 7B                                                       &7.7	&15.3	&18.7	&20.6	&15.7	&11.7	&9.1	&14.7	&9.8	&7.5	&19.5	&13.9	&10.3	&9.3	&10.1	&10.8	&12.8
                     \\
    VTimeLLM~\cite{huang2024vtimellm}                    & 7B                                                       & 37.2                  & 23.4                    & 15.0                  & \textbf{64.8}                   & 43.8                     & 53.2                   & 25.9                  & 38.8                 & 32.5                  & 25.9                  & 20.4                  & 40.9                   & 6.8                    & 48.4                  & \textbf{43.5}                    & 8.6                   & 33.1                                      \\
       \model~(Ours)                           & 4B                                                       & 56.4                  & \cellcolor{gray!30}{63.0}                    & 15.6                  & 57.1                   & \textbf{57.9}                     & \textbf{61.9}                   & \textbf{39.1}                  & 54.2                    & \textbf{73.9}                  & \cellcolor{gray!30}{41.3}                  & \cellcolor{gray!30}{29.7}                  & 92.2                   & \textbf{53.1 }                  & 69.8                  & 27.3                    & \textbf{69.9}                  & \textbf{53.9 }                                     \\
    \midrule
    \multicolumn{3}{l}{\cellcolor{gray!30}{\textit{Streaming video input at 2 fps.}}}             & \cellcolor{gray!30}{}               & \cellcolor{gray!30}{}             & \cellcolor{gray!30}{}              & \cellcolor{gray!30}{}                & \cellcolor{gray!30}{}              & \cellcolor{gray!30}{}             & \cellcolor{gray!30}{}               & \cellcolor{gray!30}{}             & \cellcolor{gray!30}{}             & \cellcolor{gray!30}{}             & \cellcolor{gray!30}{}              & \cellcolor{gray!30}{}              & \cellcolor{gray!30}{}             & \cellcolor{gray!30}{}               & \cellcolor{gray!30}{}             & \cellcolor{gray!30}{}                                 \\
    \midrule
    \textcolor{red}{VideoLLM-Online}~\cite{videollm_online}               & 7B                                                       &0	&1.8	&20.9	&5.2	&5.9	&32.6	&0	&2.3	&26.7	&0.6	&26.6	&0.9	&19.9	&0.9	&1.7	&8.3	&9.6
                     \\
    MovieChat~\cite{moviechat}                   & 7B                                                       & 23.1                  & 27.5                    & 23.6                  & 58.4                   & 43.9                     & 40.3                   & 25.6                  & 31.1                    & 23.9                  & 26.9                  & \textbf{39.6}                  & 24.4                   & 28.9                   & 29.3                  & 25.5                    & 21.9                  & 30.9                                      \\
    Flash-Vstream~\cite{flashvstream}                 & 7B                                                       & 26.9                  & 37.6                    & \textbf{23.9}                  & 60.1                   & 41.9                     & 40.0                   & 23.4                  & 35.3                    & 26.1                  & 24.7                  & 28.8                  & 27.0                   & 21.4                   & 29.8                  & 25.6                    & 26.8                  & 31.2                                      \\
  \model~(Ours)                        & 4B                                                       & \textbf{64.1}                  & \textbf{59.7}                    & 16.6                  & \textbf{63.1}                   & \textbf{58.3}                     & \textbf{62.8}                   & \textbf{42.2}                  & \textbf{54.4}                    & \textbf{70.6}                  & \textbf{54.1}                  & 24.8                  & \textbf{88.7}                   & \textbf{48.5}                   & \textbf{73.0}                  & \textbf{25.9}                    & \textbf{71.7}                  & \textbf{54.9}                                      \\
    \bottomrule
    
    \end{tabular}%
    }
    \vspace{-0.3cm}
\caption{Extra Evaluations results on \benchname. Newly reported model performance is indicated in \textcolor{red}{red}.}
\vspace{-0.3cm}
\label{tab:ov_bench_extra}
    \end{table*}
